# Supplementary material for: Topological-defect-induced surface charge heterogeneities in nematic electrolytes
Source: arXiv:2004.12833 ancillary file (2020-07-15)
Supplement: Supplementary file 1 [file SI.pdf]

# Supplemental Information: Topological-defect induced surface-charge heterogeneities in nematic electrolytes

Miha Ravnik<sup>1,2</sup> and Jeffrey C. Everts<sup>1,\*</sup>

<sup>1</sup>*Faculty of Mathematics and Physics, University of Ljubljana, Jadranska 19, 1000 Ljubljana, Slovenia*

<sup>2</sup>*Department of Condensed Matter Physics, Jozef Stefan Institute, Jamova 39, 1000 Ljubljana, Slovenia*

(Dated: May 27, 2020)

## DERIVATION OF EULER-LAGRANGE EQUATIONS

In this section we derive the Euler-Lagrange equations used for the nematic cell of the main text. The total free energy can be written as

$$\mathcal{F}[\phi, \rho_{\pm}, \mathbf{Q}] = \mathcal{F}_{\text{LC}}[\mathbf{Q}] + \mathcal{F}_{\text{I}}[\rho_{\pm}] + \mathcal{F}_{\text{EL}}[\phi, \rho_{\pm}, \mathbf{Q}] + \mathcal{F}_{\text{S}}[\mathbf{Q}], \quad (\text{S.1})$$

in terms of the tensorial nematic order parameter  $\mathbf{Q}(\mathbf{r})$ , electrostatic potential  $\phi(\mathbf{r})/(\beta q_e)$ , with  $\beta^{-1} = k_B T$  the thermal energy,  $k_B$  the Boltzmann constant,  $T$  the absolute temperature, and finally, ion densities for cations  $\rho_+(\mathbf{r})$  and anions  $\rho_-(\mathbf{r})$ .

The liquid-crystal part is described by an elastic term in the one-constant approximation, and bulk terms,

$$\mathcal{F}_{\text{LC}}[\mathbf{Q}] = \int_{\text{cell}} d\mathbf{r} \left\{ \frac{L}{2} \partial_k Q_{ij}(\mathbf{r}) \partial_k Q_{ij}(\mathbf{r}) + \frac{A}{2} \text{tr}[\mathbf{Q}(\mathbf{r})^2] + \frac{B}{3} \text{tr}[\mathbf{Q}(\mathbf{r})^3] + \frac{C}{4} \{\text{tr}[\mathbf{Q}(\mathbf{r})^2]\}^2 \right\}, \quad (\text{S.2})$$

with  $L$  the elastic constant, and  $A$ ,  $B$  and  $C$  Landau-de Gennes bulk parameters. The non-electrostatic ion contributions are treated as an ideal gas,

$$\beta \mathcal{F}_{\text{I}}[\rho_{\pm}] = \sum_{\alpha=\pm} \int_{\text{cell}} d\mathbf{r} \rho_{\alpha}(\mathbf{r}) \{ \ln[\rho_{\alpha}(\mathbf{r}) \Lambda_{\alpha}^3] - 1 \}, \quad (\text{S.3})$$

which are electrostatically coupled to each other and to  $\mathbf{Q}$  via a dielectric coupling and via flexo and order electricity,

$$\beta \mathcal{F}_{\text{EL}}[\phi, \rho_{\pm}, \mathbf{Q}] = \int_{\text{cell}} d\mathbf{r} \left[ q(\mathbf{r}) \phi(\mathbf{r}) + \nabla \phi(\mathbf{r}) \cdot \mathbf{P}_f(\mathbf{Q}(\mathbf{r})) - \frac{1}{8\pi \lambda_B \bar{\epsilon}} \epsilon_{ij}(\mathbf{Q}(\mathbf{r})) \partial_i \phi(\mathbf{r}) \partial_j \phi(\mathbf{r}) \right]. \quad (\text{S.4})$$

The total net charge density  $q(\mathbf{r})$  is given for the nematic cell as

$$q(\mathbf{r}) = \rho_+(\mathbf{r}) - \rho_-(\mathbf{r}) + \sigma(\mathbf{r}) \delta(z), \quad (\text{S.5})$$

with  $q_e \sigma(\mathbf{r})$  the net surface charge density. The flexo- and order-electric polarisation  $q_e \mathbf{P}_f$  is given in the one-constant approximation as,

$$(P_f)_i(\mathbf{r}) = G \partial_j Q_{ij}(\mathbf{r}), \quad (\text{S.6})$$

with  $q_e G$  the (molecular) flexoelectric constant. The dielectric tensor is given by

$$\epsilon_{ij}(\mathbf{r}) = \bar{\epsilon} \delta_{ij} + \frac{2}{3} \epsilon_m^a Q_{ij}(\mathbf{r}), \quad (\text{S.7})$$

with  $\bar{\epsilon}$  the isotropic dielectric constant and  $\epsilon_m^a$  the molecular dielectric anisotropy. Finally, we defined the isotropic Bjerrum length  $\lambda_B = \beta q_e^2 / (4\pi \epsilon_0 \bar{\epsilon})$ , with  $\epsilon_0$  the vacuum permittivity. The surface anchoring contribution depends on

---

\* [jeffrey.everts@gmail.com](mailto:jeffrey.everts@gmail.com)

the system in consideration. For the first nematic cell of the main text, we used homeotropic anchoring conditions for the top plate  $\Gamma_T$ , given by the Rapini-Papoular surface free energy,

$$\mathcal{F}_S[\mathbf{Q}] = \frac{W}{2} \int_{\Gamma_T} d\Gamma (Q_{ij} - Q_{ij}^0)^2, \quad (\text{S.8})$$

with  $\mathbf{Q}^0 = (3/2)S_{\text{eq}}(\mathbf{e}_z \otimes \mathbf{e}_z - \mathbf{I}/3)$  and  $W$  the anchoring strength. The boundary conditions becomes,

$$\hat{\nu}_k \beta L \partial_k Q_{ij} + \beta W (Q_{ij} - Q_{ij}^0) + G \overline{\nu_{(i} \partial_{j)} \phi} = 0, \quad (\text{S.9})$$

where round brackets around tensor indices mean symmetrisation. In contrast, for the second type of nematic cell, we use planar degenerate anchoring conditions for the top plate using the Fournier-Galatola surface free energy,

$$\mathcal{F}_S[\mathbf{Q}] = \int_{\Gamma_T} d\Gamma \left[ W_1^d (\tilde{Q}_{ij} - \tilde{Q}_{ij}^\perp)^2 + W_2^d \left( \tilde{Q}_{ij} \tilde{Q}_{ji} - \frac{9}{4} S_s^2 \right)^2 \right], \quad (\text{S.10})$$

with  $\tilde{Q}_{ij} = Q_{ij} + \delta_{ij} S_{\text{eq}}/2$  and  $\tilde{Q}_{ij}^\perp = P_{ik} \tilde{Q}_{kl} P_{lj}$ , with projection operator  $P_{ij} = \delta_{ij} - \hat{\nu}_i \hat{\nu}_j$  that projects the  $\mathbf{Q}$  tensor on the surface normal  $\hat{\nu}$ . Since we are interested in what happens on the bottom plate, we ignore surface-preferred ordering,  $S_s = S_{\text{eq}}$ . Finally,  $W_1^d$  is the in-plane anchoring strength, and  $W_2^d$  is the surface-ordering anchoring strength. This leads to the Euler-Lagrange equation,

$$\nu_k \beta L \partial_k Q_{ij} + 2\beta W_1^d \left[ \tilde{Q}_{ij} - \tilde{Q}_{ij}^\perp + \frac{\delta_{ij}}{3} \left( Q_{xx} + Q_{yy} - \frac{S_{\text{eq}}}{2} \right) \right] + 4\beta W_2^d \left( \tilde{Q}_{kl} \tilde{Q}_{kl} - \frac{9}{4} S_s^2 \right) Q_{ij} + G \overline{\nu_{(i} \partial_{j)} \phi} = 0. \quad (\text{S.11})$$

In the main text, we considered a constant surface potential  $\Phi_0$  for the bottom plate  $\Gamma_B$ , so we perform the Legendre transform

$$\mathcal{F}_\Phi[\phi, \rho_\pm, \mathbf{Q}, \sigma] = \mathcal{F}[\phi, \rho_\pm, \mathbf{Q}] - \int_{\Gamma_B} d\mathbf{r} \sigma(\mathbf{r}) \Phi_0. \quad (\text{S.12})$$

The functional derivative  $\delta \mathcal{F}_\Phi / \delta \sigma(\mathbf{r}) = 0$ , then gives the constant-potential boundary condition. The other Euler-Lagrange equations with taken into account the surface terms give rise to the Euler-Lagrange equations in the main text, where the variation with respect to  $\rho_\pm(\mathbf{r})$  should be taken in the grand-canonical ensemble and the variation over  $\mathbf{Q}(\mathbf{r})$  is taken such that  $\mathbf{Q}$  stays traceless and symmetric in the bulk and on the surfaces. Finally, for the colloidal spheres in the main text the procedure is the same, only we add an external hard-core potential so that ions cannot penetrate the particle, and that the dielectric constant inside the particle is  $\epsilon_p$ , rather than  $\epsilon_{ij}(\mathbf{r})$ .

For all the numerical calculations we use the parameters corresponding to the standard nematic liquid crystals, such as 5CB. The LdG parameters are  $A = -0.172 \cdot 10^6 \text{ J m}^{-3}$  (room temperature),  $B = -2.12 \cdot 10^6 \text{ J m}^{-3}$ ,  $C = 1.74 \cdot 10^6 \text{ J m}^{-3}$ . For elastic constants we take the one-constant approximation for simplicity and set  $L = 4 \cdot 10^{-11} \text{ J m}^{-1}$ . Dielectric properties are  $\bar{\epsilon} = 10.3$  (so  $\lambda_B = 6 \text{ nm}$ ),  $\epsilon_{\parallel}^m = 33.3$  and  $\epsilon_{\perp}^m = 12.4$  [S1], and then  $\epsilon_a^m = \epsilon_{\parallel}^m - \epsilon_{\perp}^m$ . The flexoelectric coefficients chosen in the main text are of the order of magnitude what one should expect for LCs such as 5CB [S2]. For example, within the single constant approximation,

$$q_e \mathbf{P}_f = q_e G \nabla \cdot \mathbf{Q} = \frac{3}{2} S q_e G [\mathbf{n}(\nabla \cdot \mathbf{n}) - \mathbf{n} \times (\nabla \times \mathbf{n})] + \text{order electricity terms}, \quad (\text{S.13})$$

which has to be compared with the purely flexo-electric polarisation

$$q_e \mathbf{P}_f = e_1 \mathbf{n}(\nabla \cdot \mathbf{n}) - e_3 \mathbf{n} \times (\nabla \times \mathbf{n}). \quad (\text{S.14})$$

Hence in the single-constant approximation,  $e_1 = e_3 = (3/2) S q_e G$ . In Ref. [S2] they measured at  $T = 303 \text{ K}$ ,  $e_1 + e_3 = 8.64 \text{ pC m}^{-1}$ , justifying the order of magnitude for  $q_e G$  we choose in the main text. We note that in general  $e_1 \neq e_3$  (not captured in our single-constant approximation) and there are many measurements available even for  $e_1 - e_3$  of 5CB [S3]. It would be interesting, however, to also measure the order-electric coefficients, which will become more important close to defects. In our single-constant approximation, the order electricity is, however, taken into account.

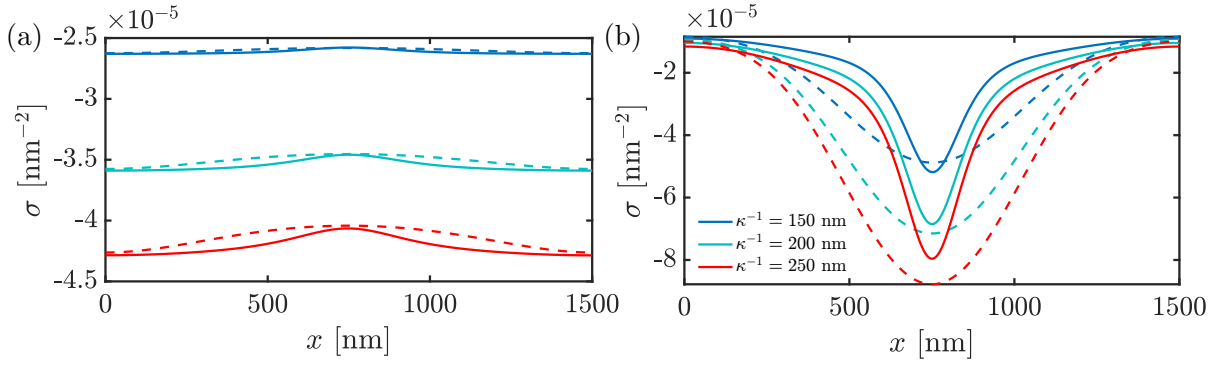

Figure S1. Effect of charge regulation on the electric double layer with a surface charge distribution  $\sigma$  on the bottom plate in the presence of a line defect in the nematic bulk. The bottom plate has equilibrium constant  $K = 1.8 \cdot 10^{-11}$  M and homeotropic anchoring is used for the top plate with  $W = 10^{-3}$  J m $^{-2}$  (dashed lines, surface defect) and  $W = 10^{-2}$  J m $^{-2}$  (full lines, bulk line defect). (a) No flexoelectricity  $G = 0$  and (b) with flexoelectricity  $G = 10$  pC m $^{-1}$ .

### GRAHAME EQUATION FOR CONSTANT-POTENTIAL AND CONSTANT-CHARGE SINGLE SURFACES

Consider a single flat plate at  $z = 0$  in an isotropic solvent, Such a system is described by the Poisson-Boltzmann (PB) equation

$$\phi''(z) = \kappa^2 \sinh[\phi(z)], \quad (\text{S.15})$$

with boundary conditions

$$\phi'(0^+) = -4\pi\lambda_B\sigma, \quad \phi'(z \rightarrow \infty) = 0, \quad (\text{S.16})$$

with  $\sigma$  fixed, or with the constant-potential boundary condition  $\phi(0^+) = \Phi_0$ . The PB equation in this geometry is analytically solvable. We multiply Eq. (S.15) with  $\phi'(z)$  to find

$$\frac{1}{2} \frac{d}{ds} \left( \frac{d\phi}{ds} \right)^2 = \frac{d}{ds} \cosh \phi, \quad (\text{S.17})$$

with dimensionless coordinate  $s = \kappa z$ . This equation is straightforward integrated to find

$$\frac{1}{2} \left( \frac{d\phi}{ds} \right)^2 = \cosh \phi + C = \cosh \phi - 1 = 2 \sinh^2[\phi(s)/2]. \quad (\text{S.18})$$

We used the global charge neutrality condition to determine the integration constant and properties of hyperbolic functions in the last step. The negative square root is compatible with the boundary condition, so we find for constant-charge and constant-potential conditions that

$$\sinh[\phi(0^+)/2] = 2\pi\lambda_B\kappa^{-1}\sigma. \quad (\text{S.19})$$

When  $\Phi_0$  is fixed or  $\sigma$  is fixed, this yields the Grahame equation

$$\sigma = \frac{1}{2\pi\lambda_B\kappa^{-1}} \sinh \left( \frac{\Phi_0}{2} \right). \quad (\text{S.20})$$

### PATTERNED SURFACES WITH LANGMUIR-ADSORPTION TYPE CHARGING

The constant-potential case is a simplification, realistic surfaces acquire their charge via the dissociation or association of ions on distinct chemical groups on the surface, such as carboxyl groups that are deprotonated  $-\text{COOH} \rightleftharpoons \text{COO}^- + \text{H}^+$ . It can be shown that such surfaces can be described by the Langmuir adsorption isotherm, see for example Ref. [S4],

$$\sigma(x, y, 0) = -\sigma_m \left\{ 1 + \frac{\rho_s}{K} \exp[-\phi(x, y, 0^+)] \right\}^{-1}, \quad (\text{S.21})$$

with  $K$  the equilibrium constant of the above reaction and  $\sigma_m$  the number density of chargeable sites on the surface. Note that such an isotherm behaves a bit differently than the constant-potential case, which acquires a higher charge for increasing  $\rho_s$  (decreasing  $\kappa^{-1}$ ). Instead, the charge becomes more negative for decreasing  $\rho_s$  (increasing  $\kappa^{-1}$ ). Using this Langmuir adsorption isotherm we solve for the pattern of Fig. 2 of the main text for the surface charge distribution in Fig. S1. Just as for the constant-potential case, the width of the surface charge distribution becomes smaller when the topological defect approaches the bottom plate. The difference is, however, that also the amplitude becomes smaller, compare with Figs. 2(c) and (f) of the main text. This shows that the manipulation by topological defects behave differently depending on the charge regulation mechanism. We would have found an enhancement of the amplitude, however, if we would have taken an associative chemical reaction where ions adsorb on the surface.

### GRAHAME EQUATION FOR LANGMUIR-TYPE SINGLE SURFACES

Although the Grahame equation holds for any type of Langmuir adsorption isotherm, it is not a priori known what the surface potential is given the material parameters (such as equilibrium constant(s) or screening lengths). However, we can derive Grahame-like expressions also for these adsorption isotherms in terms of  $K$  and  $\rho_s$ , which we shall do for the reaction mechanism of the previous section. Our starting point is Eq. (S.19) and we insert Eq. (S.21),

$$-\sinh[\phi(0^+)/2] = 2\pi\lambda_B\kappa^{-1}\sigma_m \left\{ 1 + \frac{\rho_s}{K} \exp[-\phi(0^+)] \right\}^{-1}, \quad (\text{S.22})$$

where we assumed here isotropic solvents.

In the limit where  $\sigma \ll \sigma_m$  a simple analytical solution exists for  $\phi(0^+)$ . The system is transformed to

$$-\sinh[\phi(0^+)/2] = \gamma \exp[\phi(0^+)], \quad (\text{S.23})$$

with  $\gamma = 16\pi^2\lambda_B^2\kappa^{-3}K\sigma_m$ . This equation can be rewritten with the variable  $\ln x = -\phi(0^+)/2$  (note  $\phi(0^+) < 0$ ), as

$$-2\gamma x^3 + x^2 - 1 = 0, \quad (\text{S.24})$$

with discriminant of this cubic equation

$$\Delta = 4 - 108\gamma^2. \quad (\text{S.25})$$

Based on the discriminant, we have either 3 real roots for  $\Delta > 0$  or 1 real root and 2 complex roots (that are each others complex conjugate) for  $\Delta < 0$ . We are interested in solutions that are real and where  $x > 0$ . Using the Viète solution of a cubic equation, we find

$$\phi(0^+) = 2 \ln \left\{ -\frac{1}{6\gamma} + \frac{1}{3\gamma} \cos \left[ \frac{1}{3} \arccos(54\gamma^2 - 1) \right] \right\}, \quad \sigma \ll \sigma_m. \quad (\text{S.26})$$

Hence the surface charge density is

$$\sigma = \frac{\sigma_m K}{\rho_s} \left\{ -\frac{1}{6\gamma} + \frac{1}{3\gamma} \cos \left[ \frac{1}{3} \arccos(54\gamma^2 - 1) \right] \right\}^2, \quad \sigma \ll \sigma_m. \quad (\text{S.27})$$

From this formula we can directly see the increase of the surface charge density upon increasing  $\kappa^{-1}$ , in contrast to the constant-potential case discussed in the main text.

### AVERAGE SURFACE CHARGE DENSITY AND SURFACE CHARGE AMPLITUDE

In Figs. 2(d) and (f) in the main text we show the surface charge density profiles comparing a boojum (surface defect) on the top uncharged plate with a line bulk defect, with and without flexoelectricity, for various screening lengths  $\kappa^{-1}$ . Furthermore, it was mentioned in the main text that the average surface charge density is approximately described by the Grahame equation. To show this, we expand Figs. 2(d,f) into Fig. S2(a,c) showing that even in the flexoelectric case the average surface charge density,

$$\bar{\sigma} = \frac{1}{w} \int_0^w dx \sigma(x), \quad (\text{S.28})$$

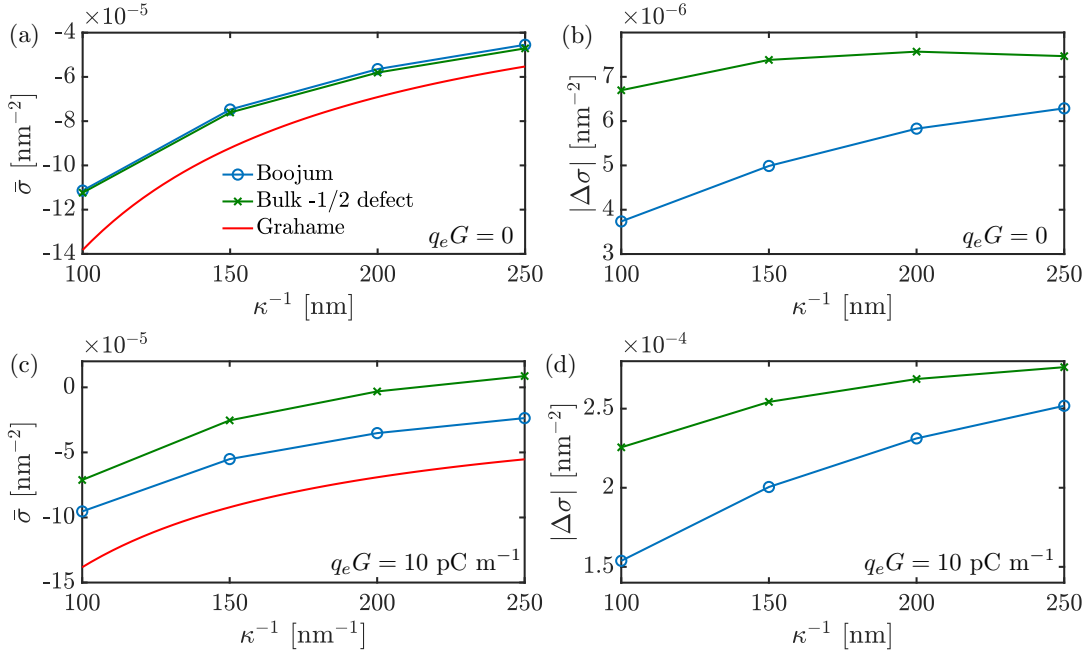

Figure S2. Average surface charge density  $\bar{\sigma}$  and surface charge amplitude  $|\Delta\sigma|$  for the cases plotted of Fig. 2 in the main text. We highlight the differences between Boojum (surface) defect and a bulk line defect with winding number  $-1/2$ , with and without flexoelectricity. Note for  $\bar{\sigma}$  the comparison with the Grahame equation Eq. (S.20).

is reasonably described by the Grahame equation Eq. (S.20), thus to good degree capturing the qualitative trend as function of  $\kappa^{-1}$ . The accuracy of this approximation for  $\bar{\sigma}$  is expected to be better for smaller double layers such that the large separation assumption which underlies Eq. (S.20) is satisfied.

Furthermore, in Figs. S2(b,d) we show the dependence of the surface charge amplitude defined by

$$\Delta\sigma = \max_{x \in [0, w]} \sigma(x) - \min_{x \in [0, w]} \sigma(x) \quad (\text{S.29})$$

as function of  $\kappa^{-1}$  showing that larger surface charge inhomogeneities are present for the bulk line defect for all the  $\kappa^{-1}$  that we considered in the main text. Recall also that  $\sigma(x)$  becomes more strongly peaked around  $x = w/2$  for this specific patterned surface for a bulk line defect that is closer to the bottom plate.

Regarding the above analysis it is relevant to replot Fig. S1 for the Langmuir adsorption isotherm Eq. (S.21), see Fig. S3. We compare  $\bar{\sigma}$  with the modified Grahame equation (S.27) that is derived for an ion-dissociation electrostatic boundary condition on the bottom plate, showing again good qualitative agreement, with and without flexoelectricity [see Figs. S3(a,c)]. For  $|\Delta\sigma|$  and  $G = 0$  the amplitudes are comparable for the bulk and surface defect, with a slightly higher amplitude for a bulk defect. Which amplitude is bigger depends on  $\kappa^{-1}$  for  $G \neq 0$ , sometimes the bulk defect gives a larger  $|\Delta\sigma|$ , sometimes the boojum. However, in all cases, as clearly evident from Fig. S3,  $\sigma$  is more strongly peaked for the bulk defect.

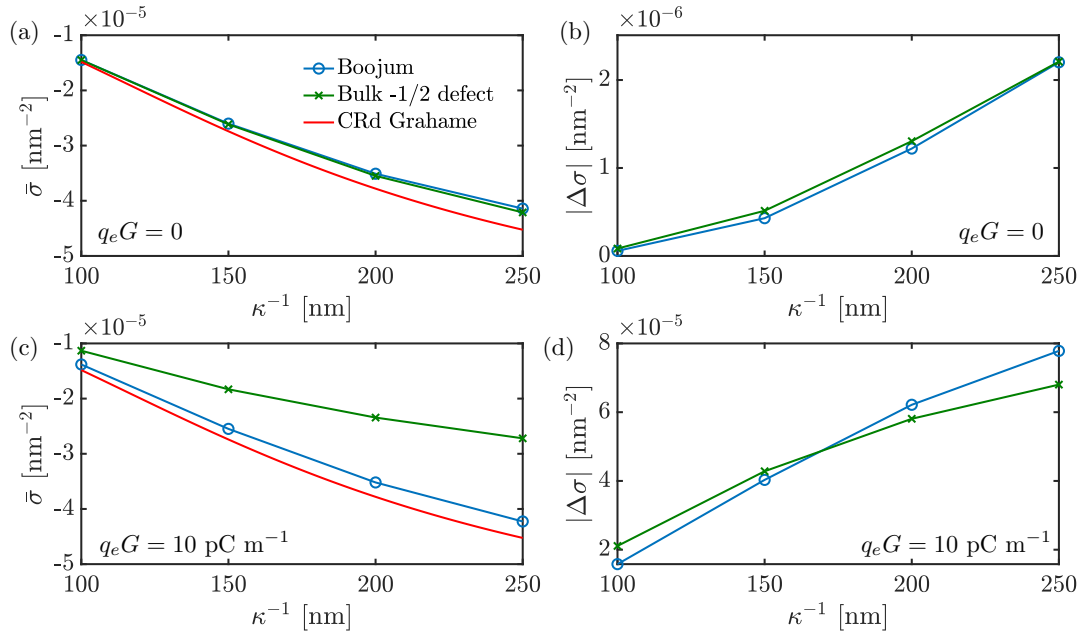

Figure S3. Average surface charge density  $\bar{\sigma}$  and surface charge amplitude  $|\Delta\sigma|$  for the cases plotted of Fig. S1. We highlight the differences between Boojum (surface) defect and a bulk line defect with winding number  $-1/2$ , with and without flexoelectricity. Note for  $\bar{\sigma}$  the comparison with the modified Grahame equation Eq. (S.27).

- 
- [S1] A. Bogi and S. Faetti, *Liq. Cryst.* **28**, 729 (2001).  
[S2] P. R. M. Murthy, V. A. Raghunathan, and N. V. Madhusudana, *Liq. Cryst.* **14**, 483 (1993).  
[S3] F. Castles, S. C. Green, D. J. Gardiner, S. M. Morris, and H. J. Coles, *AIP Adv.* **2**, 022137 (2012).  
[S4] N. Boon and R. van Roij, *J. Chem. Phys.* **134**, 054706 (2011).
